# Supplementary material for: Online Learning and Information Exponents: On The Importance of Batch size, and Time/Complexity Tradeoffs
Source: arXiv:2406.02157 source file (2024-06-04)
Supplement: Supplementary file 1 [file simple_explanation.tex]

\section{Informal Explanation to be trashed (rigor is taken care of in Appendix B)}
\label{sec:app:to_read}
The key idea of this work is to give a Pareto-like trade-off between the training time $T$ and the batch size $n_b$ for learning a target function $f^\star$ with a teacher-student network. The main result is given in Theorem \ref{thm:main:} and states that the relation between the training time $T$ and the batch size $n_b$. We detail here informally the ida behind the derivation. 

\paragraph*{Common assumptions} We assume Hermite polynomial activations for the teacher and student networks. More precisely, we assume that the teacher and student networks have the same Hermite polynomial activation of degree $s$. Moreover, consider for simplicity one hidden neurons ($p=1$), single-index targets ($k=1$), fixed learning rate $\gamma$, and spherical dynamics ($Q_\tau = 1)$.

\paragraph*{Learning rate bounds:} 
There are two bounds on the learning rate that needs to be satisfied: 
\begin{itemize}
    \item \textbf{Martingale bound:} The learning rate $\gamma$ needs to satisfy the martingale bound $\gamma < \gamma_{\rm{mart}}$. This bounds accounts for the fact that the noise contribution is negligible, we set the threshold for negligibility by asking that the cumulative effect of the noise terms is comparable to the initial condition randomness. The reasoning is very similar to \cite{arous2021online} [Equation 1.8]. 
    \begin{align}
        m_{\tau + 1} = m_\tau + \gamma_{\tau} \beta_{\ell} m_{\tau}^{\ell - 1} - \gamma_\tau \Xi_{\tau}
    \end{align}
    The noise factor $\Xi_{\tau}$ is the correction to the gradient descent on the population loss. After $T$ steps, the cumulative effect of the noise terms can be informally written as: 
    \begin{align}
        \Xi_{\rm{cum}} &= \gamma \sum_{\tau = 1}^T \Xi_{\tau} \approx \gamma \frac{1}{n_b}\sum_{\tau = 1}^T \sum_{\nu = 1}^{n_b} \xi_{\tau}^{\nu} \\
        &= \frac{\gamma \sqrt{T}}{\sqrt{n_b}} 
    \end{align}
    We call $\gamma_{\rm{mart}}$ the learning rate threshold for which the cumulative effect of the noise terms is comparable to the initial condition randomness - $m_0 \sim \frac{1}{\sqrt{d}}$:
    \begin{align}
        \gamma_{\rm{mart}} \sqrt{\frac{T}{n_b}} \simeq \frac{1}{\sqrt{d}}
        \label{eq:gamma_martingale}
    \end{align}
    \item \textbf{Stability bound:} The learning rate $\gamma$ needs to satisfy the stability bound $\gamma < \gamma_{\rm{stab}}$. This bounds accounts for the fact that the dynamics of the sufficient statistics $m$ is \textit{unstable} around the uninformative fixed point $m = 0$. 
\end{itemize}

\paragraph*{Example of computation of the stability bound - $n_b = 1$} This bound can be computed in detail by considering one simple case the well studied case $n_b = 1$ \cite{arous2021online,arnaboldi.stephan.ea_2023_high}. We can study the stability of the uninformative fixed point by expanding the equations around $m =0$. We obtain the following linearized system (we divide the learning rate by $d$ to be coherent with \cite{arnaboldi.stephan.ea_2023_high}, i.e., $\gamma = \frac{\gamma_0}{d}$):
\begin{align}
    \dod{m}{t} = -\alpha_s \gamma_0 m + \beta_s m^{s-1} + \gamma_0 o(m) - o(m^{s-1})
\label{eq:stability_zero_fp_hermite_s_nb=1}
\end{align}
where \(\frac{\alpha_s}{s^2 s!}\) and \(\beta_s\) are costant depnding just on \(s\): \[\beta_s = s!s \qquad \alpha_s = \{1,3,32,642,18624,703440,\cdots\}\]
We note that the general structure has an expansive term $\beta_s m^{s-1} + \gamma_0o(m)$, and a contractive one $\alpha_s\gamma_0 m + o(m^{s-1})$. The trade off between these two quantities will determine the dynamics.
\paragraph*{Retrieving GBA information exponent:} By studying eq.~\eqref{eq:stability_zero_fp_hermite_s} we see that in order to be able to escape mediocrity we need:  \begin{align}
    \gamma_0 < \frac{\alpha_s}{\beta_s}m_0^{s-2}
    \label{eq:app:stability_bound_ss}
\end{align}
    We are interested in retrieving what is the sample complexity for learning such single-index targets $\text{He}_s$. The sample complexity can be written as:
    $$n_{tot} = \frac{t_{esc}}{\frac{\gamma_0}{d}} = O_d\left(t_{esc} \frac{1}{\gamma_0} d\right)$$ We can compute the time to escape mediocrity $t_{esc}$ by solving the equation: 
    \begin{align}
        \dod{m}{t} = C m^{s-1} \qquad m(0) =m_0.
    \end{align}
    with \(C>0\) given the condition on \(\gamma_0\). If we define \(t_\text{esc}\) as the time needed to escape a threshold \(T: m(t_{esc}) = T\), then 
    \[
     t_\text{esc}(m_0) = 
     \begin{cases}
        \label[type]{eq:escaping_times}
        \frac{T-m_0}{C} & \text{if } s = 1 \\
        \frac{\log\left(\frac{T}{m_0}\right)}{C} & \text{if } s = 2 \\
        \frac{1}{C(s-2)}\left(\frac{1}{m_0^{s-2}} - \frac{1}{T^{s-2}}\right) & \text{if } s > 2
     \end{cases}
    \]
    The initialization we use implies that \(m_0 = O\left(\frac{1}{\sqrt{d}}\right)\) when \(d\to\infty\). We can then compute the sample complexity for all the information exponents:
    \begin{itemize}
        \item \textbf{s=1}: here \(t_\text{esc} = O(1)\) and no condition on \(\gamma_0\), so the overall sample complexity is \(n_{tot} = O(d)\).
        \item \textbf{s=2}: here \(t_\text{esc} = O(\log{d})\) and \(\gamma_0 = O(1)\) with the condition \(\gamma_0 < \sfrac{\beta_2}{\alpha_2} = \sfrac16\) so the overall sample complexity is \(n_{tot} = O(d\log{d})\), as we have already seen in escaping mediocrity paper (including the bound on \(\gamma_0\)!).
        \item \textbf{$s>2$}: here \(t_\text{esc} = O(d^\frac{s-2}{2})\) and \(\gamma_0 = O(d^\frac{2-s}{2})\), so the overall sample complexity is \[n_{tot} = O(d^\frac{s-2}{2} \frac{1}{d^\frac{2-s}{2}} d ) = O(d^{s-1}).\]
    This matches the findings of \cite{arous2021online}.
    \end{itemize}

\paragraph*{Martingale bound form} The expression for the learning rate $\gamma_{\rm{mart}}$ in eq.~\eqref{eq:gamma_martingale} can be rewritten in the following form by assuming that the training time $T$ will respect the functional form in eq.~\eqref{eq:escaping_times} ($\gamma < \gamma_{\rm{stab}}$):
\begin{align}
    T \sim \frac{1}{\gamma}(\frac{1}{m_0})^{s-2} 
\end{align}  
By plugging this expression for the time steps inside eq.~\eqref{eq:gamma_martingale} we obtain: 
\begin{align}
    \gamma_{\rm{mart}} \sim n_b d^{\frac{-s}{2}}
    \label{eq:app:martingale_bound_nb_general}
\end{align}

\subsection{The role of $\hat{y}$ interaction term}
Unfortunately, a naive and wrong reasoning has misled us: we were assuming that the same phenomenology happening at $n_b = 1$ would have gone through for general batch sizes. 
\\ This was a reasonable assumption, as a careful analysis of the main terms would have agreed with this conclusion. 
\\ However, there is one term that is easily neglected, but apparently crucial for the analysis of cold start learning: the terms in the decomposition of the gradient including $\hat{y}$, i.e., the prediction term.
{\color{blue} {
\paragraph{Wrong reasoning presented here just for clarity and for collaborator to catch up --} the Pareto-frontier is given by the relation $\log_dT + \log_dn_b = s - 1$. Indeed, neively we could just require that the iteration time $T$ becomes $O(1)$ - Assuming that $\gamma = \gamma_{\rm{mart}} < \gamma_{\rm{stab}}$ and we obtain:
\begin{align}
    T_{\rm{crit}} &= \frac{1}{\gamma_{\rm{mart}}}(\frac{1}{m_0})^{s-2} \\
    &= \frac{d^{s-1}}{n_b} = O(1)
\end{align}

The critical batch size would be close to $n_b = d^{s-1}$.  }}

\paragraph{Correct reasoning --} In constrast with the GiantStep paper, we CANNOT neglect the term coming from $\hat{y}$ if we are interested in studying the dynamics under the condition: a) starting from cold start $m_{t=0} = \varepsilon << 1 $; b) $n_b < d^{\ell}$, i.e., the dynamics will be iterated for at least $\log{T}$ time step. 

\paragraph{Careful expansion of equations with cold start $\forall n_b$ -- } Let us consider the dynamics of projected SGD and expand it for small values of the initial correlation $m_0$ without fixing the batch size $n_b$. As in the previous section we fix the teacher-student network to have matching architecture, by fixing the information exponent $\text{IE} = s$. We obtain the following: 
\begin{align}
    m_{t+1} \simeq \gamma \beta_s (m_t)^{s-1} -\gamma^2 m_t \left(\frac{\alpha_s d}{n_b} + f_s \right) + \text{H.O.T}
    \label{eq:app:expansion_cold_start_nb_generic}
\end{align}

The quantities $(\alpha_s, \beta_s)$ are appearing already in the $n_b = 1$ case illustrated in eq.~\eqref{eq:stability_zero_fp_hermite_s_nb=1}. However, a new term represented by $f_s$ appears in the expansion: this term represents an interaction given by the presence of the prediction term $\hat{y}$. 
\\ More precisely we can identify the contribution of $f_s$ as the one coming from this term in the Saad \& Solla equations: 
\begin{align}
\mathbb{E}\left[\sigma'(\lambda_j)\mathcal E (\lambda^\bot)^\top\right]\left(Q^\bot\right)^{-1}\mathbb{E}\left[\sigma'(\lambda_l)\mathcal E \lambda^\bot\right]
\end{align}
Note, that the equation above is present only for $n_b=1$, so the $\hat{y}$ terms are not relevant in the $n_b=1$ case also if $\hat{y}\neq 0$.
\paragraph{Conseqeucnces of this term into the Pareto frontier reasoning --} 

By analyzing eq.~\eqref{eq:app:expansion_cold_start_nb_generic} different regimes will appear that modify the original Pareto frontier reasoning: 
\begin{itemize}
    \item If we consider batch sizes $n_b <d$ we note  that the $f_s$ term is going to be killed. In this case the relationship $\log{T} + \log{n_b} = s-1$ is still valid if we choose the critical learning rate: 
    $$\gamma_{\text{crit}} = O( n_b d^{-s/2}) \to d^{-\delta} = d^k d^{-s/2}  $$
    This leads us to the First part of the phase diagram in Fig. 1 (to complete): 
    \begin{align}
        \delta_\text{crit} = \frac{s}{2} - k
        \label{eq:app:stab1}
    \end{align}
    The line given by eq.~\eqref{eq:app:stab1} is the solid green line in Fig.~\ref{fig:phase_diagrams} appearing for $n_b <d$. 
    \item If we consider batch sizes $n_b >d$ the term associated to $f_s$ is dominant. This term is a contractive term that is not dependent on the batch size. This will break the Pareto frontier reasoning:
    \begin{align}
        \gamma_\text{crit} = O(d^{-s/2 + 1})
    \end{align}
    Leading to:
    \begin{align}
        \delta_{\text{crit}} = \frac{s}{2} - 1
        \label{eq:app:stab2}
    \end{align}
    We cannot increase anymore the learning rate and the time complexity $T$ does not respect anymore the original Pareto frontier line $\log{T} + \log{n_b} = s-1$, i.e., the relation on the exponent given in eq.~\eqref{eq:app:stab1}. 
    \\ The line identified by eq.~\eqref{eq:app:stab2} is the solid horizontal line in Fig.~\ref{fig:phase_diagrams}.
\end{itemize}

\paragraph{Removing the interaction by rescaling the 2nd layer --} Thanks to the above analysis we are able to theoretically understand when the term $f_s$ in eq.~\eqref{eq:app:expansion_cold_start_nb_generic} will be relevant. Indeed, since this term is derived from the prediction term $\hat{y}$, we could suppress it by assuming a smaller scaling for the $2$nd layer $\vec a \in \mathbb{R}^p$! 
Unfortunately, we are not able to observe with true simulations the theoretically plausible positive effect in the escape from mediocrity. 
\\ If we remove artificially the term associated to $\hat{y}$,  the stability line in the phase diagram \ref{fig:phase_diagrams} is the dashed green line. 
\paragraph{Warm start learning --} If we consider a finite non-vanishing value of the initial correlation $m_0$ we are able to expand the Saad \& Solla closed form equations and identify a phase diagram similar to [Veiga et al.] just by analyzing which terms vanish / dominate in the high-dimensional limit. This idea has been agreed after a joint meeting to be a secondary message with respect the cold start learning regime.  

\section{DUmp of all notes}
\subsection{Analytical cases}
We move now to particular cases in which the integrals are computable analytically. 
\paragraph{Analytic case \# 1: $\text{He}_2$}
We now rewrite the equations using the choice: 
$$\sigma (z)= \sigma^* (z)= \text{He}_2(z) = z^2 - 1$$
We compute the auxiliary functions defined in eq.~\eqref{eq:define_Is} and we report them in Appendix~\ref{sec:app:H2_theory}
\textbf{Takehome messages}: We fix for the analysis $k=p=1$, and we call $M_{11} = m$.
\begin{itemize}
    \item \textbf{Online SGD:} Same result as the escaping mediocrity paper. The constant does not matter for the information exponent. We note that the fixed point $m = 0$ is contractive if $\gamma_0 \geq \frac 16$.
    \item \textbf{Large batch SGD:}
    The time necessary to escape from mediocrity is \(T = O(\log{d})\). This is in accordance with the results of the online case, given that the total sample complexity is \(n_{tot} = O(d\log{d})\). We note that the fixed point $m = 0$ is contractive if $\gamma_0 \geq  0.125$.
\end{itemize}

\paragraph{Analytic case \# 2: \(\text{He}_3\)}
We now rewrite the equations using the choice: 
$$\sigma (z)= \sigma^* (z)= \text{He}_3(z) = z^3 - 3z$$
We compute the auxiliary functions defined in eq.~\eqref{eq:define_Is} and we report them in Appendix~\ref{sec:app:theory_H3}. 
\textbf{Takehome messages}:
We fix for the analysis $k=p=1$, and we call $M_{11} = m$.
\begin{itemize}
     \item \textbf{Online SGD:} We note empirically that the bacin of attraction of $m=0$ is much larger. More precisely, we see that for small initial correlation $m^{t=0} = \varepsilon$, the learning rate must be respect $\gamma_0 \leq C_{\rm{ON}} \varepsilon$.
    \item \textbf{Large batch SGD:}
    Same phenomenology as the online case. However, the learning rate must respect $\gamma_0 \leq C_{\rm{LB}}\varepsilon$. 
\end{itemize}
These two auxiliary quantities $C_{\rm{ON}},C_{\rm{LB}}$ are constant not depending on the dimension $d$ but only on the degree of the polynomial $s$. We refer to the next section in which we unveil the general dependencies for any Hermite polynomial.
\paragraph{Analytic case \# 2: \(\text{He}_3\) -- Expansion to find information exponent \(s\)}
Looking at the results above, we understand that the stability of the $m=0$ fixed point governs the dynamics. In principle we can write down explicitly the equation for any polynomial activation (with the help of a Mathematica code), but they are huge. For simplicity we also use the spherical version of the online SGD algorithm, where \(M_{11}\) is the only sufficient parameter describing the problem. For brevity, we define \(m\equiv M_{11}\). The leading order of the ODE governing the online SGD dynamics is:
\begin{align}
    \dod{m}{t} = -\alpha_s \gamma_0 m + \beta_s m^{s-1} + \gamma_0o(m) -o(m^{s-1})
\label{eq:stability_zero_fp_hermite_s}
\end{align}
where \(\alpha_s\) and \(\beta_s\) are costant depnding just on \(s\): \[\beta_s = s!s \qquad \alpha_s = \{1,3,32,642,18624,703440,\cdots\}\]
We note that the general structure has an expansive term $\beta_s m^{s-1} + \gamma_0o(m)$, and a contractive one $\alpha_s\gamma_0 m + o(m^{s-1})$. The trade off between these two quantities will determine the dynamics. \textbf{Takehome messages}:
\begin{itemize}
    \item \textbf{Retrieving GBA information exponent:} By studying eq.~\eqref{eq:stability_zero_fp_hermite_s} we see that in order to be able to escape mediocrity we need:  $$\gamma_0 < \frac{\alpha_s}{\beta_s}m_0^{s-2}.$$
    We are interested in retrieving what is the sample complexity for learning such single-index targets $\text{He}_s$. The sample complexity can be written as:
    $$n_{tot} = \frac{t_{esc}}{\frac{\gamma_0}{d}} = O_d\left(t_{esc} \frac{1}{\gamma_0} d\right)$$ We can compute the time to escape mediocrity $t_{esc}$ by solving the equation: 
    \begin{align}
        \dod{m}{t} = C m^{s-1} \qquad m(0) =m_0.
    \end{align}
    with \(C>0\) given the condition on \(\gamma_0\). If we define \(t_\text{esc}\) as the time needed to escape a threshold \(T: m(t_{esc}) = T\), then 
    \[
     t_\text{esc}(m_0) = 
     \begin{cases}
        \frac{T-m_0}{C} & \text{if } s = 1 \\
        \frac{\log\left(\frac{T}{m_0}\right)}{C} & \text{if } s = 2 \\
        \frac{1}{C(s-2)}\left(\frac{1}{m_0^{s-2}} - \frac{1}{T^{s-2}}\right) & \text{if } s > 2
     \end{cases}
    \]
    The initialization we use implies that \(m_0 = O\left(\frac{1}{\sqrt{d}}\right)\) when \(d\to\infty\). We can then compute the sample complexity for all the information exponents:
    \begin{itemize}
        \item \textbf{s=1}: here \(t_\text{esc} = O(1)\) and no condition on \(\gamma_0\), so the overall sample complexity is \(n_{tot} = O(d)\).
        \item \textbf{s=2}: here \(t_\text{esc} = O(\log{d})\) and \(\gamma_0 = O(1)\) with the condition \(\gamma_0 < \sfrac{\beta_2}{\alpha_2} = \sfrac16\) so the overall sample complexity is \(n_{tot} = O(d\log{d})\), as we have already seen in escaping mediocrity paper (including the bound on \(\gamma_0\)!).
        \item \textbf{$s>2$}: here \(t_\text{esc} = O(d^\frac{s-2}{2})\) and \(\gamma_0 = O(d^\frac{2-s}{2})\), so the overall sample complexity is \[n_{tot} = O(d^\frac{s-2}{2} \frac{1}{d^\frac{2-s}{2}} d ) = O(d^{s-1}).\]
    This matches the findings of GBA.
    \end{itemize}
    \item \textbf{Optimal learning rate:} We predict $\forall s$ an optimal learning rate to use. However, if we reason on the $s=1$ case, and we perfmorm the computation, we see that the optimal learning rate is $\gamma_0 = \sqrt{d}$ (starting from the differential equation \eqref{eq:stability_zero_fp_hermite_s}). This would yield a sample complexity (that depends on the time unit and hence $\gamma_0$) better than GBA. More precisely: $\text{US} \sim \sqrt{d}$ vs $\text{GBA} \sim d$.
    \item \textbf{Benefit of overapametrization} WE can guess from the structor of the equation that the benefit of overparametrization could play a significant role when \(s>2\), in contrast with Escaping mediocrity paper, where the effect on \(s=2\) is only mild. We need to repeat this derivation for generic \(p\). 
    \item \textbf{Large-batch SGD} The same procedure can be repeated for the spherical version of the large batch SGD case, without chaning the qualitative behaviour but only the sequences defining $(\alpha_s,\beta_s)$.
\end{itemize}

\subsection{Benefit of overparametrization}

\subsection{Does stochasticity matter?}

\subsection{}

\section*{TO-DO}
 \begin{itemize}
    \item Check numerics in an extensive way. SS equations are not guaranteed to work for $T$ large. First on online spherical SGD and then the other three. 
    \item Make explicit the fact that there are many thresholds on the learning rate. 
    \item Write the analytical expression of large batch spherical SGD. 
    \item Are there any relevant stochastic corrections? If so, compute the SDE in these cases.
     \item Study population landscape 
     \item Quantify benefit of overparametrization 
     \item Quantify critical magnetization as a function of the learning rate $\gamma$.
     \item What is the rationale to avoid detrimental effect of $I_4$ overparametrization.  
     \item Dynamics of staircase function. We cannot consider high polynomials as the equations quickly increase their complexity. However, we might try: 
     \begin{enumerate}
         \item 
     SS Plot to show that using staircase function (eg $f^\star_1 = \lambda^\star_1 + \lambda^\star_1 \lambda^\star_2 + \lambda^\star_1 \lambda^\star_2 \lambda^\star_3$) the rank of the projected weights increases at every iteration (approximately). 
    \item SS Plot to show that rank increase does not happen fdor finite number of GD step using function which is non-staircasable in the $n=O(d)$ regime, (eg $f^*_2 (\lambda^*) = \lambda^*_1 + \lambda^*_1\text{He}_2(\lambda^*_2) + \lambda^\star_1 \lambda^\star_2 \lambda^\star_3 $). 
    \end{enumerate}
    \item Dynamics in the $n = O(d^s)$ polynomial regime is dependent on $d$. How to fix?
 \end{itemize}

% Manual newpage inserted to improve layout of sample file - not
% needed in general before appendices/bibliography.

\newpage
